# Supplementary material for: SPOCK: A proximal method for multistage risk-averse optimal control problems
Source: arXiv:2212.01110 source file (2022-12-02)
Supplement: Supplementary file 1 [file appendix.tex]

\section{Dynamic programming (DP) for $\proj_{\mS_1}$}
\label{app_stochastic}

\subsection{Defining value functions}
Define the leaf value function $V^{\star i}_0(x^i;\xb^i) = \tfrac{1}{2}\|x^i-\xb^i\|^2, \forall i\in\nodes(N)$. Define the nonleaf value function
\begin{multline}\label{eq:define-Vtplus1}
    V_{t+1}^{\star i}(x^i; \xb^i,\ub^i,\xb^{i_+}) = 
    \minimise_{\substack{x^i, u^i\\i\in\nodes(N-(t+1))}}
    \\
    \tfrac{1}{2}\Big( \|x^i-\xb^i\|^2 + \|u^i-\ub^i\|^2 \Big)
    \\
    {}+{}
    \sum_{i_+\in\ch(i)}\ 
    \underbracket[0.5pt]{
    \tfrac{1}{2}\|
    \left(A^{i_+}x^i + B^{i_+}u^i\right)
    -\xb^{i_+}\|^2}_{V_t^{\star i}(x^{i_+}; \bar{x}^{i_+})},
\end{multline}
for $t\in\N_{[0, N-1]}$, $i\in\nodes(N-(t+1))$ and $i_+\in\ch(i)$. We now assume that $V_{t+1}^{\star i}(x^{i})$ is quadratic and has the general form
\begin{equation}\label{eq:quadratic-form}
    V_{t+1}^{\star i}(x^{i}) = \tfrac{1}{2}x^{i\intercal} P^i_{t+1} x^i + q_{t+1}^{i\intercal} x^i + c^i_{t+1}.
\end{equation}
Indeed, $V_0^{\star i}$ can be written as above,
\begin{align}
    V^{\star i}_0(x^i;\xb^i) 
    {}={}& 
    \tfrac{1}{2}x\iTop x^i - \xb\iTop x^i + \tfrac{1}{2}\|\xb^i\|^2,
\end{align}
where $P_0 = I$, $q_0^i = -\xb^i$ and $c_0^i = \tfrac{1}{2}\|\xb^i\|^2$.

\subsection{Finding the gradient of the nonleaf value function w.r.t. the control action, $u^i$}
From Equation \eqref{eq:define-Vtplus1} and the assumption from Equation \eqref{eq:quadratic-form}
\begin{multline}\label{eq:Vtplus1-long}
    V_{t+1}^{\star i}(x^i;\xb^i,\ub^i) 
    {}={}%
    \minimise_{\substack{x^i, u^i\\i\in\nodes(N-(t+1))}}
    \\
    \underbracket[.5pt]{
    \tfrac{1}{2}\Big( \|x^i-\xb^i\|^2 + \|u^i-\ub^i\|^2 \Big)}_{\text{Part1}}
    \\[.5em]
    {}+{} \sum_{i_+\in\ch(i)}\ \Big( \underbracket[.5pt]{ \tfrac{1}{2}
    \left(A^{i_+}x^i + B^{i_+}u^i\right)\Top P^{i_+}_{t} \left(A^{i_+}x^i + B^{i_+}u^i\right)}_{\text{Part2}}
    \\[.5em]
    {}+{} \underbracket[.5pt]{
    q^{i_+\intercal}_{t} \left(A^{i_+}x^i + B^{i_+}u^i\right) + c^{i_+}_{t}}_{\text{Part3}} \Big),
\end{multline}
for $t\in\N_{[0, N-1]}$, $i\in\nodes(N-(t+1))$ and $i_+\in\ch(i)$. We take the gradient of the value function above w.r.t $u^i$, and set the result equal to zero, which yields
\begin{multline}
    \nabla_{u^i} V^i_{t+1}
    {}={}
    0
    {}={}%
    u^i - \ub^i 
    \\
    + \sum_{i_+\in\ch(i)} \left( B^{i_+\intercal} P^{i_+}_{t} \left( A^{i_+}x^i + B^{i_+}u^i \right) + B^{i_+\intercal} q^{i_+}_{t}  \right),
\end{multline}
therefore, $\widetilde{R}_{t+1} = I + \sum_{i_+\in\ch(i)} B^{i_+\intercal} P^{i_+}_{t} B^{i_+}$ and
\begin{multline}
    \kappa_{t+1}^{\star i}(x^i)
    {}={}
    \underbracket[0.5pt]{
    \widetilde{R}_{t+1}^{-1}
    \left(
    - \sum_{i_+\in\ch(i)} B^{i_+\intercal} P^{i_+}_{t} A^{i_+}
    \right)
    }_{K^i_{t+1}} x^i
    \\
    + \underbracket[0.5pt]{
    \widetilde{R}_{t+1}^{-1}
    \left(
    \ub^i - \sum_{i_+\in\ch(i)} B^{i_+\intercal} q^{i_+}_{t}
    \right),
    }_{d^i_{t+1}}
\end{multline}
for $t\in\N_{[0, N-1]}$, $i\in\nodes(N-(t+1))$ and $i_+\in\ch(i)$.

\subsection{Evaluating nonleaf value functions, $V^{\star i}_{t+1}$ }
Let us define $\Ab^{i_+}_{t+1} = A^{i_+} + B^{i_+}K^i_{t+1} = \Ab$. From Equation \eqref{eq:Vtplus1-long}, when $u^i = \kappa^{\star i}_{t+1}(x^i) = K^i_{t+1}x^i + d^i_{t+1}$,
\begin{multline}
    V_{t+1}^{\star i}(x^i;\xb^i,\ub^i) 
    {}={}
    \minimise_{\substack{x^i, u^i\\i\in\nodes(N-(t+1))}}
    \\
    \underbracket[.5pt]{
    \tfrac{1}{2}\left( \|x^i-\xb^i\|^2 + \|(K^i_{t+1}x^i + d^i_{t+1}) -\ub^i\|^2 \right)
    }_{\text{PartA$^i$}}
    \\
    \sum_{i_+\in\ch(i)}\ \Big( \underbracket[.5pt]{ \tfrac{1}{2}
    \left(\Ab x^i + B^{i_+} d^i_{t+1}\right)\Top P^{i_+}_{t} \left(\Ab x^i + B^{i_+} d^i_{t+1}\right)
    }_{\text{PartB$^i$}}
    \\
    {}+{}
    \underbracket[.5pt]{
    q^{i_+\intercal}_{t} \left(\Ab x^i + B^{i_+} d^i_{t+1}\right) + c^{i_+}_{t}
    }_{\text{PartC$^i$}}
    \Big),
\end{multline}
for $t\in\N_{[0, N-1]}$, $i\in\nodes(N-(t+1))$ and $i_+\in\ch(i)$. Expanding and rearranging finally results in

\begin{multline}
    V_{t+1}^{\star i}(x^i;\xb^i,\ub^i) 
    {}={}
    \tfrac{1}{2} 
    x\iTop \left(
    I + K_{t+1}^{i\intercal} K^i_{t+1} + \bar{A}\Top P^{i_+}_t \bar{A}
    \right) x^i
    \\
    + \Bigg[
    K_{t+1}^{i\intercal} \left( d_{t+1}^i - \ub^i \right)
    - \xb^i
    \\
    + \sum_{i_+\in\ch(i)} \bar{A}\Top \left( P^{i_+}_t B^{i_+} d_{t+1}^i + q^{i_+}_t \right)
    \Bigg]\Top x^i
    \\
    + 
    \tfrac{1}{2} \left(
    \|\xb^i\|^2 + \|d_{t+1}^i - \ub^i\|^2
    \right) 
    \\
    + \sum_{i_+\in\ch(i)} \left( \tfrac{1}{2}
    d_{t+1}^{i\intercal} B^{i_+\intercal} P^{i_+}_t B^{i_+} d_{t+1}^i
    + q^{i_+\intercal}_t B^{i_+} d_{t+1}^i
    + c^{i_+\intercal}_t
    \right)
\end{multline}

that is
\begin{subequations}\label{app:stochastic-update-eqns}
\begin{align}
    \widetilde{R}_{t+1}^i {}={}&
    I 
    + \sum_{i_+\in\ch(i)} B^{i_+\intercal} P^{i_+}_{t} B^{i_+}
    \\
    K_{t+1}^i {}={}&
    -\widetilde{R}_{t+1}^{-1}
    \sum_{i_+\in\ch(i)} B^{i_+\intercal} P^{i_+}_{t} A^{i_+},
    \\
    d_{t+1}^i {}={}&
    \widetilde{R}_{t+1}^{-1}
    \left( 
    \ub^i - \sum_{i_+\in\ch(i)} B^{i_+\intercal} q^{i_+}_{t}
    \right),
    \\
    \bar{A}_{t+1}^{i_+} {}={}&
    A^{i_+} + B^{i_+}K^i_{t+1}, \forall i_+ \in\ch(i),
    \\
    P_{t+1}^i {}={}& 
    I + K_{t+1}^{i\intercal} K^i_{t+1} + \bar{A}\Top P^{i_+}_t \bar{A}
    \\
    q_{t+1}^i {}={}&
    K_{t+1}^{i\intercal} \left( d_{t+1}^i - \ub^i \right)
    - \xb^i
    \\
    & + \sum_{i_+\in\ch(i)} \bar{A}\Top \left( P^{i_+}_t B^{i_+} d_{t+1}^i + q^{i_+}_t \right)
\end{align}
\end{subequations}
for $t\in\N_{[0, N-1]}$, $i\in\nodes(0, N-1)$, $i_+\in\ch(i)$ and with initial conditions $P^i_0=I, q^i_0=-\xb^i, \forall i\in\nodes(N)$. We have omitted $c^i_{t+1}$.
